# Supplementary material for: Self-Supervised Attention Learning for Depth and Ego-motion Estimation
Source: arXiv:2004.13077 source file (2022-12-05)
Supplement: Supplementary file 1 [file 7_Appendix.tex]

\appendix \chapter{Appendix} 
\section{Implementation Details}
\subsubsection{DispNet}

\begin{table}[H]
  \centering
  \resizebox{\linewidth}{!}{
  \begin{tabular}[t]{|l|l|l|l|l|l|l|}
\hline
\multicolumn{7}{|l|}{\textbf{``Encoder''}} \\
\hline
\textbf{layer} & \textbf{k} & \textbf{s} & \textbf{chns} & \textbf{in} & \textbf{out} & \textbf{input}       \\ \hline
cnv1         & 7               & 2               & 3/32              & 1              & 2               & target                 \\
cnv1b        & 7               & 1               & 32/32             & 2              & 2               & cnv1                \\
cnv2         & 5               & 2               & 32/64             & 2              & 4               & cnv1b               \\
cnv2b        & 5               & 1               & 64/64             & 4              & 4               & cnv2                \\
cnv3         & 3               & 2               & 64/128            & 4              & 8               & cnv2b               \\
cnv3b        & 3               & 1               & 128/128           & 8              & 8               & cnv3                \\
cnv4         & 3               & 2               & 128/256           & 8              & 16              & cnv3b               \\
cnv4b        & 3               & 1               & 256/256           & 16             & 16              & cnv4                \\
cnv5         & 3               & 2               & 256/512           & 16             & 32              & cnv4b               \\
cnv5b        & 3               & 1               & 512/512           & 32             & 32              & cnv5                \\
cnv6         & 3               & 2               & 512/512           & 32             & 64              & cnv5b               \\
cnv6b        & 3               & 1               & 512/512           & 64             & 64              & cnv6                \\
cnv7         & 3               & 2               & 512/512           & 64             & 128             & cnv6b               \\
cnv7b        & 3               & 1               & 512/512           & 128            & 128             & cnv7                \\ \hline
\end{tabular}
\begin{tabular}[t]{|l|l|l|l|l|l|l|}
\hline
\multicolumn{7}{|l|}{\textbf{``Decoder''}} \\
\hline
\textbf{layer} & \textbf{k} & \textbf{s} & \textbf{chns} & \textbf{in} & \textbf{out} & \textbf{input}       \\ \hline
upcnv7       & 3               & 2               & 512/512           & 128            & 64              & cnv7b               \\
icnv7        & 3               & 1               & 1024/512          & 64             & 64              & upcnv7+cnv6b        \\
upcnv6       & 3               & 2               & 512/512           & 64             & 32              & icnv7               \\
icnv6        & 3               & 1               & 1024/512          & 32             & 32              & upcnv6+cnv5b        \\
upcnv5       & 3               & 2               & 512/256           & 32             & 16              & icnv6               \\
icnv5        & 3               & 1               & 512/256           & 16             & 16              & upcnv5+cnv4b        \\ \hline
upcnv4       & 3               & 2               & 256/128           & 16             & 8               & icnv5               \\
icnv4        & 3               & 1               & 128/128           & 8              & 8               & upcnv4+cnv3b        \\
disp4        & 3               & 1               & 128/1             & 8              & 8               & icnv4               \\ \hline
upcnv3       & 3               & 2               & 128/64            & 8              & 4               & icnv4               \\
icnv3        & 3               & 1               & 129/64            & 4              & 4               & upcnv3+cnv2b+disp4  \\
disp3        & 3               & 1               & 64/1              & 4              & 4               & icnv3               \\ \hline
upcnv2       & 3               & 2               & 64/32             & 4              & 2               & icnv3               \\
icnv2        & 3               & 1               & 65/32             & 2              & 2               & upcnv2+cnv1b+disp3  \\
disp2        & 3               & 1               & 32/1              & 2              & 2               & icnv2               \\ \hline
upcnv1       & 3               & 2               & 32/16             & 2              & 1               & icnv2               \\
icnv1        & 3               & 1               & 17/16             & 1              & 1               & upcnv1+disp2        \\
disp1        & 3               & 1               & 16/1              & 1              & 1               & icnv1               \\ \hline
\end{tabular}  }
  \vspace{0pt}
\caption{DispNet architecture, where \textbf{k} is the kernel size, \textbf{s} the stride, \textbf{chns} the number of input and output channels for each layer, \textbf{in}put and \textbf{out}put is the downscaling factor for each layer relative to the input image, and \textbf{input} corresponds to the input of each layer where $+$ is a concatenation. Upsampling is done by convolution transpose.}
\label{tab:DispNet}
\vspace{-10pt}
\end{table}

\subsubsection{Pose/ExpNet}
\begin{table}[H]
  \centering
  \resizebox{\linewidth}{!}{
  \begin{tabular}[t]{|l|l|l|l|l|l|l|}
\hline
\multicolumn{7}{|l|}{\textbf{``Encoder - PoseNet''}} \\
\hline
\textbf{layer} & \textbf{k} & \textbf{s} & \textbf{chns} & \textbf{in} & \textbf{out} & \textbf{input}       \\ \hline
cnv1         & 7               & 2               & 3*(1+S)/16        & 1              & 2               & target+ nearby     \\
cnv2         & 5               & 2               & 16/32             & 2              & 4               & cnv1               \\
cnv3         & 3               & 2               & 32/64             & 4              & 8               & cnv2               \\
cnv4         & 3               & 2               & 64/128            & 8              & 16              & cnv3               \\
cnv5         & 3               & 2               & 128/256           & 16             & 32              & cnv4               \\
cnv6         & 3               & 2               & 256/256           & 32             & 64              & cnv5               \\
cnv7         & 3               & 2               & 256/256           & 64             & 128             & cnv6               \\
pose_pred    & 1               & 1               & 256/S*6           & 128            & 128             & cnv7               \\ \hline
\end{tabular}
\begin{tabular}[t]{|l|l|l|l|l|l|l|}
\hline
\multicolumn{7}{|l|}{\textbf{``Decode - ExpNet Extension''}} \\
\hline
\textbf{layer} & \textbf{k} & \textbf{s} & \textbf{chns} & \textbf{in} & \textbf{out} & \textbf{input}       \\ \hline
upcnv5               & 4               & 2               & 256/128           & 32             & 16              & conv5            \\
upcnv4               & 4               & 2               & 128/164           & 16             & 8               & upconv5          \\
upcnv3               & 4               & 2               & 64/32             & 8              & 4               & upconv4          \\
upcnv2               & 4               & 2               & 32/16             & 4              & 2               & upconv3          \\
upcnv1               & 4               & 2               & 16/8              & 2              & 1               & upconv2          \\ \hline

predict\_mask4       & 3               & 1               & 128/S             & 8              & 8               & upconv4          \\ 
predict\_mask3       & 3               & 1               & 64/S              & 4              & 4               & upconv3          \\
predict\_mask2       & 3               & 1               & 32/S              & 2              & 2               & upconv2          \\
predict\_mask1       & 3               & 1               & 16/S              & 1              & 1               & upconv1          \\ \hline
\end{tabular} 
 }
  \vspace{0pt}
\caption{Pose/ExpNet architecture, where \textbf{k} is the kernel size, \textbf{s} the stride, \textbf{chns} the number of input and output channels for each layer, \textbf{in}put and \textbf{out}put is the downscaling factor for each layer relative to the input image, and \textbf{input} corresponds to the input of each layer where $+$ is a concatenation. Upsampling is done by convolution transpose.}
\label{tab:PoseNet}
\vspace{-10pt}
\end{table}

\subsubsection{Attention U-Net}
\begin{table}[H]
  \centering
  \resizebox{\linewidth}{!}{
  \begin{tabular}[t]{|l|l|l|l|l|l|l|}
\hline
\multicolumn{7}{|l|}{\textbf{``Encoder''}} \\
\hline
\textbf{layer} & \textbf{k} & \textbf{s} & \textbf{chns} & \textbf{in} & \textbf{out} & \textbf{input}       \\ \hline
cnv1         & 3               & 1               & 3/64              & 1              & 1               & target              \\
cnv1b        & 7               & 1               & 64/64             & 1              & 1               & cnv1                \\
cnv2         & 5               & 1               & 64/128            & 2              & 2               & cnv1b               \\
cnv2b        & 5               & 1               & 128/128           & 2              & 2               & cnv2                \\
cnv3         & 3               & 1               & 128/256           & 4              & 4               & cnv2b               \\
cnv3b        & 3               & 1               & 256/256           & 4              & 4               & cnv3                \\
cnv4         & 3               & 1               & 256/512           & 8              & 8               & cnv3b               \\
cnv4b        & 3               & 1               & 512/512           & 8              & 8               & cnv4                \\
cnv5         & 3               & 1               & 512/1024          & 16             & 16              & cnv4b               \\
cnv5b        & 3               & 1               & 1024/1024         & 16             & 16              & cnv5                \\ \hline
\end{tabular}
\begin{tabular}[t]{|l|l|l|l|l|l|l|}
\hline
\multicolumn{7}{|l|}{\textbf{``Decoder''}} \\
\hline
\textbf{layer} & \textbf{k} & \textbf{s} & \textbf{chns} & \textbf{in} & \textbf{out} & \textbf{input}       \\ \hline
up5          & 3               & 2               & 512/256           & 16             & 8               & conv5b              \\
att5         & 3               & 1               & 512/256           & 8              & 8               & up5,cnv4b           \\ 
upcnv5       & 3               & 1               & 512/256           & 8              & 8               & att5+up5            \\ \hline

up4          & 3               & 2               & 256/128           & 8              & 4               & conv4b*             \\
att4         & 3               & 1               & 128/128           & 4              & 4               & up4,cnv3b           \\
upcnv4       & 3               & 1               & 128/128           & 4              & 4               & att4+up4            \\ \hline

up3          & 3               & 2               & 128/64            & 4              & 2               & conv3b*             \\
att3         & 3               & 1               & 128/64            & 2              & 2               & up3,cnv2b           \\
upcnv3       & 3               & 1               & 128/64            & 2              & 2               & att3+up3            \\ \hline

up2          & 3               & 2               & 64/32             & 2              & 1               & conv3b*             \\
att2         & 3               & 1               & 64/32             & 1              & 1               & up2,cnv1b           \\
upcnv2       & 3               & 1               & 64/32             & 1              & 1               & att2+up2            \\ \hline

disp4        & 3               & 1               & 512/1             & 8              & 8               & upcnv5              \\
disp3        & 3               & 1               & 256/1             & 4              & 4               & upcnv4              \\
disp2        & 3               & 1               & 128/1             & 2              & 2               & upcnv3              \\
disp1        & 3               & 1               & 64/1              & 1              & 1               & upcnv2              \\ \hline
alpha4       & 3               & 1               & 1/2               & 8              & 8               & att5(alpha)         \\
alpha3       & 3               & 1               & 1/2               & 4              & 4               & att4(alpha)         \\
alpha2       & 3               & 1               & 1/2               & 2              & 2               & att3(alpha)         \\
alpha1       & 3               & 1               & 1/2               & 1              & 1               & att2(alpha)         \\ \hline
\end{tabular} }
  \vspace{0pt}
\caption{Attention U-Net architecture, where \textbf{k} is the kernel size, \textbf{s} the stride, \textbf{chns} the number of input and output channels for each layer, \textbf{in}put and \textbf{out}put is the downscaling factor for each layer relative to the input image, and \textbf{input} corresponds to the input of each layer where $+$ is a concatenation. * is a downsampled by factor of 2 using maxpooling. "up" means normal upsampling by interpolation and then a convolution. "upconv" means two convolution layers in the decoder }
\label{tab:U-Net}
\vspace{-10pt}
\end{table}

\section{Training parameters}
\begin{itemize}
    \item Smooth loss parameter: $\lambda_{smooth} = 0.1$
    \item Explainability loss parameter: $\lambda_{exp} = 0.1$ (the same for attention mask)
    \item Adversarial loss parameter: $\lambda_{GAN} = 0.5$
    \item Back loss parameter: $\lambda_{BF} = 0.5$
    \item Optimizer used: Adam Optimizer
    \begin{itemize}
        \item Learning rate: $\alpha = 0.0002$
        \item The exponential decay rate for the first moment: $\beta_1 = 0.5$
        \item The exponential decay rate for the second-moment: $\beta_2 = 0.999$
    \end{itemize}
    \item number of training epochs: 26 epochs/
    \item batch size per training iteration: 4 examples.
\end{itemize}
